# Supplementary material for: The Excess Proton at the Air-Water Interface: The Role of Instantaneous Liquid Interfaces
Source: arXiv:1703.09395 ancillary file (2017-03-28)
Supplement: Supplementary file 1 [file Supplementary_information.pdf]

# Supplemental Information: The Excess Proton at the Air-Water Interface: The Role of Instantaneous Liquid Interfaces

March 27, 2017

Federico Giberti[1], Ali A. Hassanali[2],

**1** The University of Chicago, Institute For Molecular Engineering, 5640 South Ellis Avenue, Chicago, Illinois 60637, USA.
**2** The Abdus Salam International Centre for Theoretical Physics, Condensed Matter and Statistical Physics, Strada Costiera 11, 34151 Trieste, Italy * gibertif@uchicago.edu

# 1 Computational Methods

## 1.1 Construction of the air-water interface

Two different approaches have been used to identify the position of the air-water interface: the Gibbs Dividing Interface (GDI) and the Willard Chandler Interface (WCI). In the former, the average position of the interface is obtained by calculating the water density profile as a function of the coordinate normal to the interface, $y$ in this case, and locating the surface where $\rho(y) = \rho_G(y) = 0.5$. Once that the position of the interface is define, it is relatively straightforward to calculate a probability density function of the proton position with respect to $\rho_G(y) = 0.5$.

In the WCI approach, a coarse-grained density is obtained by summing Gaussian kernels centered on each water molecule, so that $\rho(\mathbf{r}) = \sum_i^N (\sqrt{2\pi\sigma^2})^{-1} e^{-\frac{(\mathbf{r}-\mathbf{R}_i)^2}{2\sigma^2}}$, with $\sigma$=2.4 Å. The position of an instantaneous interface is then identified so that $\rho(\mathbf{r}) = \rho_{WC}(\mathbf{s}) = 0.5$. As described in the paper of Willard *et al.*, a density profile as a function of the distance from the interface can be recovered as

$$\rho(d_{WCI}) = \frac{1}{L^2} \left\langle \sum_i^N \delta(d_{WCI} - d^i_{WCI}) \right\rangle \tag{1}$$

with $d^i_{WCI}$ being:

$$d^i_{WCI} = (\mathbf{s}(t) - \mathbf{r}_i(t)) \cdot \mathbf{n}(t) \tag{2}$$

where $\mathbf{s}(t)$ is the closest point to atom $i$ belonging to the surface, and $\mathbf{n}$ is the normal of the interface calculated in that point[1].

## 1.2 Construction of the hydrogen bond network

In the ensuing analysis, we examine features of the hydrogen bond network such as the density of defective water molecules (those that deviate from accepting and donating two h-bonds) as well as topological properties like the directed proton wires. To do so, we use a standard geometrical criterion for the hydrogen bond proposed by Chandler[2]: a pair of oxygen atoms ($O_1$ and $O_2$) are considered hydrogen bonded if the distance between them is less than 3.5 Å and the H-$O_1$–$O_2$ angle is less than 30 degrees. Using this geometrical criterion, the position of the excess proton is identified as the oxygen donating 3 hydrogen-bonds to its neighboring water molecules. Using this definition of hydrogen bond, the whole system can be mapped to a graph where the vertices are the oxygen atoms which are directly linked if a hydrogen bond exists between them. This allows an easy calculation of different topological quantities that can be used to represent in a simple way, the complexity of the hydrogen bond network.

To describe the properties of the network, we define the dimension and the route of the different paths. In the ensuing analysis, all the paths are determined based on the shortest directed path between two nodes. The dimension $n$, is the number of vertexes composing the path which is equal to the number of water molecules. The route $\eta$ is a function of the geodesic distance connecting the first and last vertexes of the path, and is calculated as $\eta = \sum_i^{n-1} d(O_i, O_{i+1})$ where the sum runs over all the oxygens composing the path. Finally, $d$ is the head-to-tail Euclidean distance of the wire (head is the first water molecule that basically hosts the proton in the path, and tail is the last water molecule in the path) and $a$ is how far the water molecule at the end of the path is from the WCI.

To understand how the presence of the air-water interface alters the network, we have determined the distributions P($\eta$,$a$) and P($d$,$a$) both of which quantify the probability of finding a directed path connecting a water molecule at a distance $d$ or $\eta$ from the hydronium ion and position $a$ from the WCI.

# 2 Proton wires.

## 2.1 Coiled nature of the proton wires.

In the main text we pointed out that the proton wires are coiled. The extent of how coiled a wire can be depends of course on its length. In S1A) we have reported the probability of finding proton wires of different length characterized by a end to end distance $d$ and a geodesic distance $\eta$. For proton wires that would be perfectly linear or straight, there would be sharp and distinct peaks where $d = \eta$. Instead we see that the for longer wires, the peaks get broader.

Another way to appreciate this is to examine the distribution of $\chi = \frac{\eta}{d}$ as a function of $\eta$. This is shown in S1B). For $\chi = 1$, the proton wires are perfectly linear - it is clear that as the wires get longer, they are more coiled.

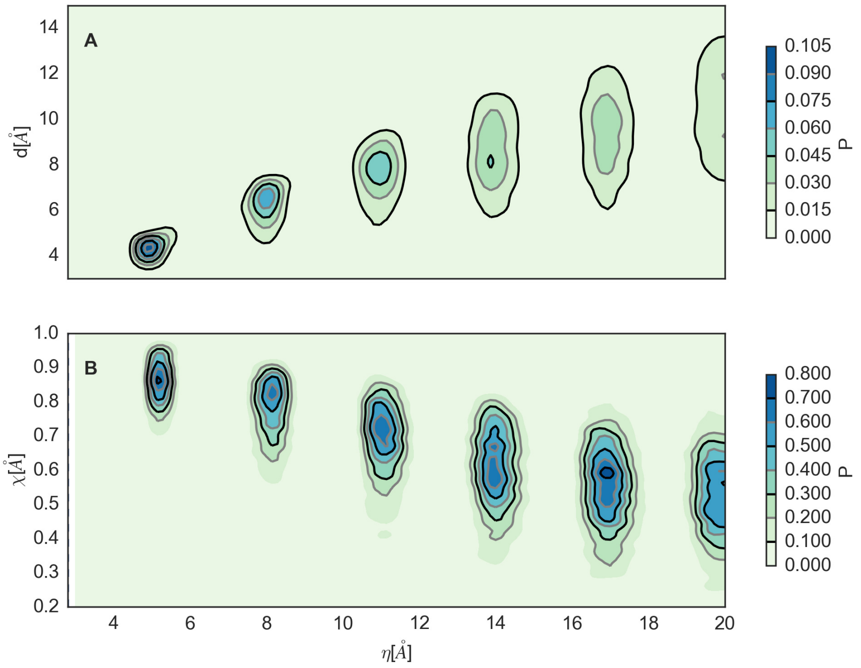


Figure S1: Coilness of the proton wires in simulation A-D, expressed as the ration between the geodesic distance and the end-to-end distance $\chi = \frac{\eta}{d}$ (panel B) ). Panel A) illustrate how the geodesic distance $\eta$ changes as a function of the euclidean distance $d$.

## 2.2 Simulation B: Water Network for Proton Trapped in the Bulk

In the main text we showed that for simulation A there were proton wires running parallel to the surface (see Figure 2 in the main text). To illustrate that simulation A was not a special case, we also determined similar distributions for simulation B. The probability as a function of the distance from the WCI is illustrated in S2A) and B). We see here that the distributions are very similar.

## 2.3 Water wires around water molecules in simulation A and D

In the main text, we alluded to the fact that the presence of proton wires running parallel to the surface was not a specific feature to the environment of the proton. In particular, we find that neutral water molecules at the surface also bear similar features and is thus a rather general feature of the network. See Fig S3 and S4 which show for two different water molecules at the surface.

A similar conclusion is reached when examining the water distribution for water molecules in the bulk. See FigureS5 and FigureS6 which resemble those for the proton in simulation D shown in the main text.

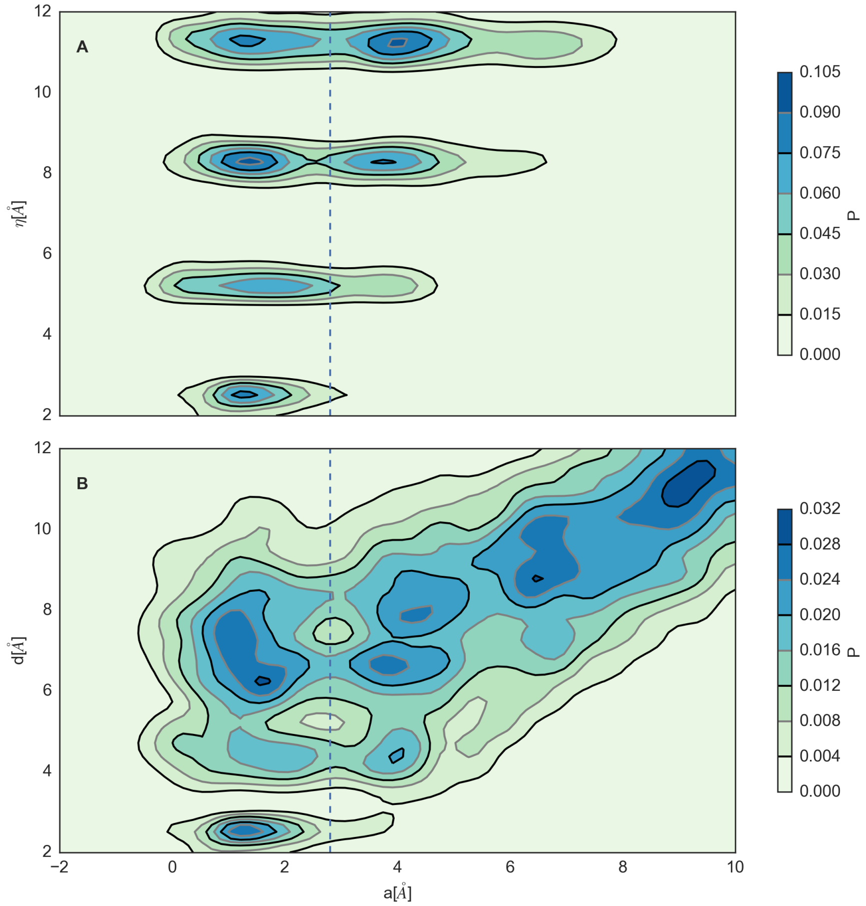


Figure S2: Probability density function of finding directed proton wire able to shuttle the excess proton at the surface or in the bulk, starting from the air-water interface. In panel A) the probability is expressed as a function of the WCI distance $a$ and the geodesic $\eta$, while in panel B the same probability is reported as a function of $a$ and the end to end distance of the proton wire $d$.

# 3 Dynamics of the excess proton in simulation A-D.

As anticipated in the text, the four simulations A-D reveal very different dynamical behavior of the proton. The mean square displacement (MSD) for the four simulations are reported in Figure S7. Simulation A and B, where the proton is equilibrated at the air-water interface, exhibit much smaller MSD compared to simulation C and D.

Simulations C and D, are characterized by much larger MSD values. In the former, the proton starts from the bulk and migrates during the simulation until it gets to the surface. The latter, is the only system where the proton remains in the bulk and appears to be undergoing lateral diffusion.

We have also quantified the decorrelation time associated with the relaxation

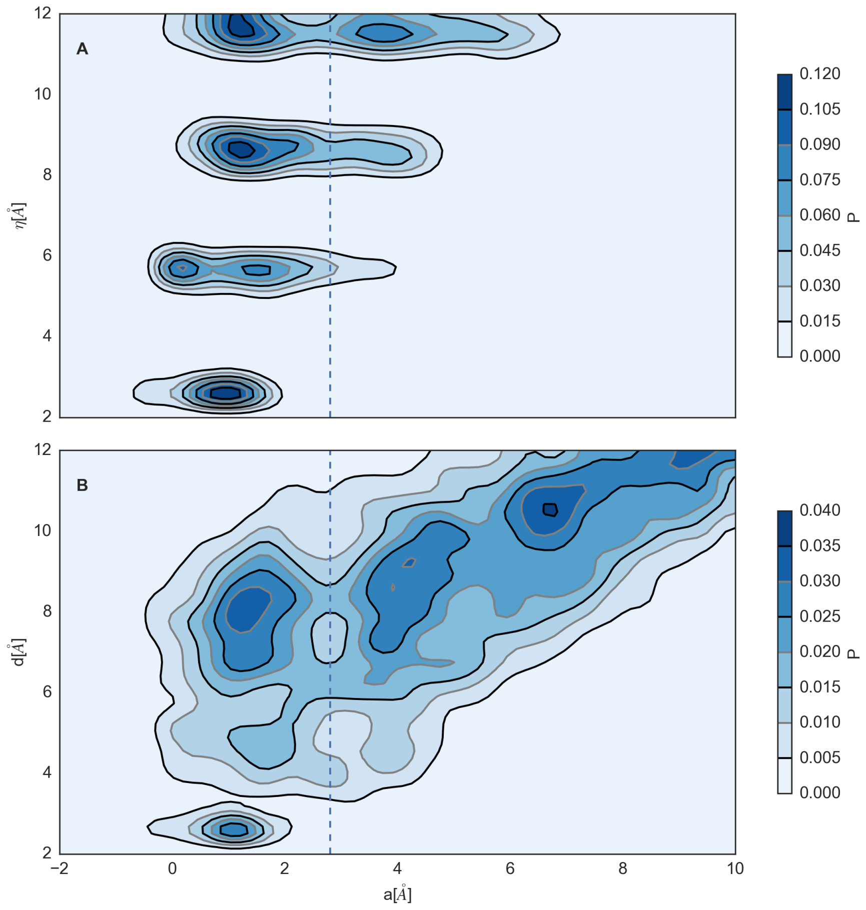


Figure S3: Panel A: probability of finding a water wire of length $\eta$ joining a water molecule at the interface and the other at distance $a$ from the interface. Panel B: probability of finding a directed water wire joining two water molecules at distance $d$ between them, when the end of the path is at distance $a$ from the WCI (panel A) ).

of water wires of different length. The calculation of the decorrelation function has been explained in the methods section of the main manuscript. The function used to fit the decay is:

$$f = Ae^{-\frac{t}{\tau_1}} + Be^{-\frac{t}{\tau_2}} \tag{3}$$

The parameters obtained from the fitting have been reported in table 3.

Due to the initial fast decay of the functions, the initial 0.5 ps have been discarded, as they increase the noise in the fitting. Fitting with more than two exponential decays did not result in any improvement of the fitted parameters.

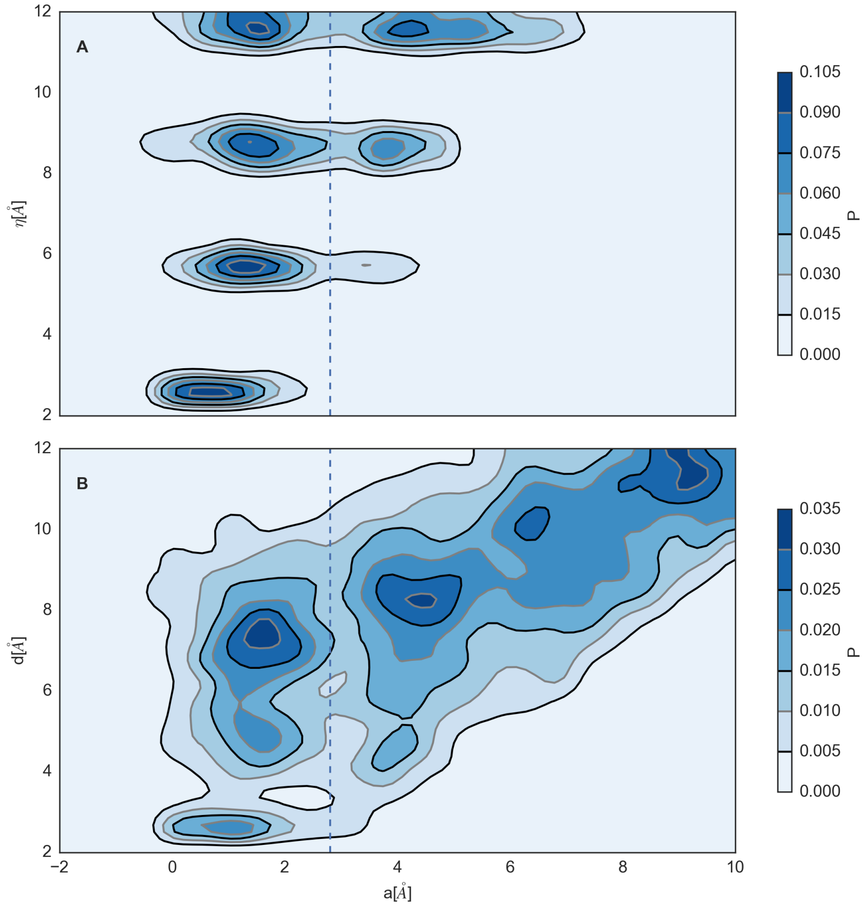


Figure S4: Panel A: probability of finding a water wire of length $\eta$ joining a water molecule at the interface and the other at distance $a$ from the interface. Panel B: probability of finding a directed water wire joining two water molecules at distance $d$ between them, when the end of the path is at distance $a$ from the WCI (panel A) ).

# 4 Coordination defects along proton wires of different length.

In the main text, we reported the probability of finding a certain topological defects as a function of the distance along a proton wires of length 1 and 4. Here we have reported the full statistic of the coordination defects along path of length 1 to 4 for simulation A and simulation D. For the proton at the surface (simulation A) ) there is a striking difference for the coordination defects in the first solvation shell (e.g. path length equal to 1), with a high probability of finding a 1in-2out defect that in the bulk. In the latter case, there is no difference between the concentration of 1in-2out at 1 hydrogen bond or 4 hydrogen bond from the hydronium ion.

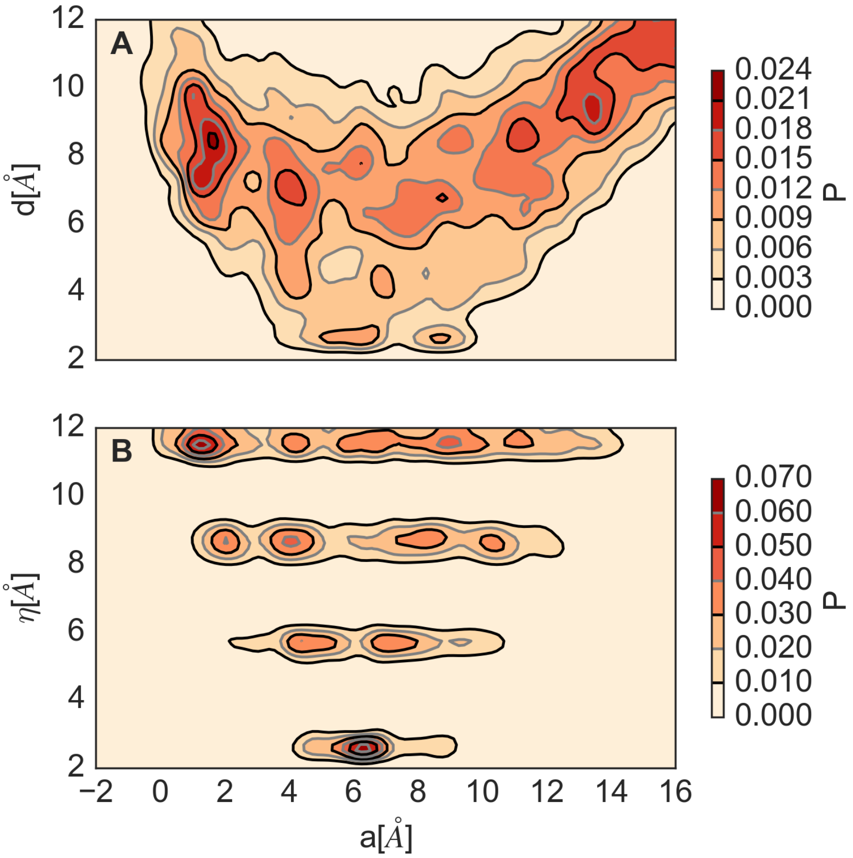


Figure S5: Panel A: probability of finding a water wire of length $\eta$ joining a water molecule in the bulk and the other at distance $a$ from the interface. Panel B: probability of finding a directed water wire joining two water molecules at distance $d$ between them, when the end of the path is at distance $a$ from the WCI (panel A) ) and the beginning is in the bulk of the slab.

## References

[1] Adam P. Willard and David Chandler. Instantaneous liquid interfaces. *J. Phys. Chem. B*, 114(5):1954–1958, 2010. PMID: 20055377.

[2] Alenka Luzar and David Chandler. Hydrogen-bond kinetics in liquid water. *Nature*, 379(6560):55–57, Jan 1996.

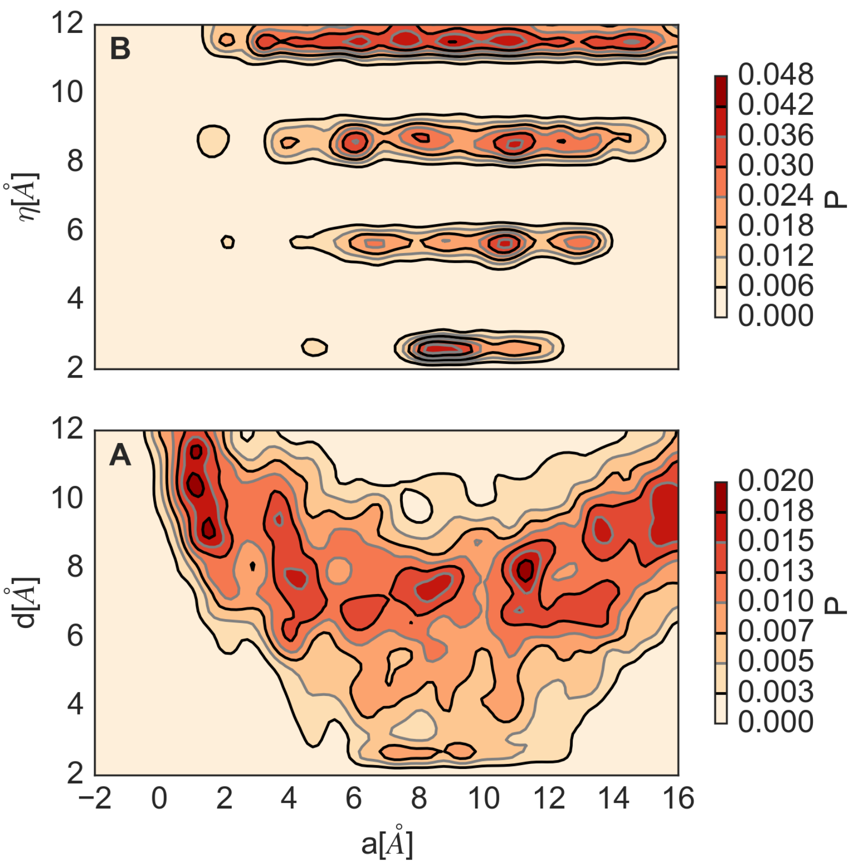


Figure S6: Panel A: probability of finding a water wire of length $\eta$ joining a water molecule in the bulk and the other at distance $a$ from the interface. Panel B: probability of finding a directed water wire joining two water molecules at distance $d$ between them, when the end of the path is at distance $a$ from the WCI (panel A) and the beginning is in the bulk of the slab.

Table S1: Lifetime of different water wires calculated by fitting the decorrelation function reported in the main manuscript

| Defect | A | $\tau_1$ [ps] | B | $\tau_2$ [ps] |
|---|---|---|---|---|
| path 1 | 0.190 | 1.197 | 0.739 | 34.676 |
| path 2 | 0.192 | 1.407 | 0.734 | 36.356 |
| path 3 | 0.227 | 2.072 | 0.687 | 56.052 |
| path 4 | 0.201 | 1.526 | 0.747 | 57.231 |

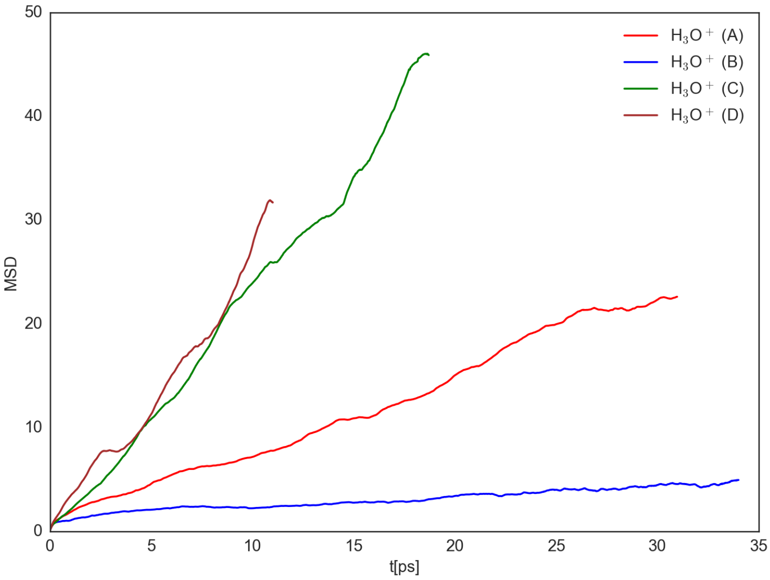


Figure S7: Mean Square Displacements for the four hydronium ions of simulations A, B, C and D. While we were expecting to observe to see a difference between the proton buried in the bulk and those at the surface, but to our surprise even proton A and B show a remarkable difference. This behavior once more confirms that caution needs to be employed when calculating the diffusion coefficient of the excess proton, as even small starting conditions may produce different trajectories.

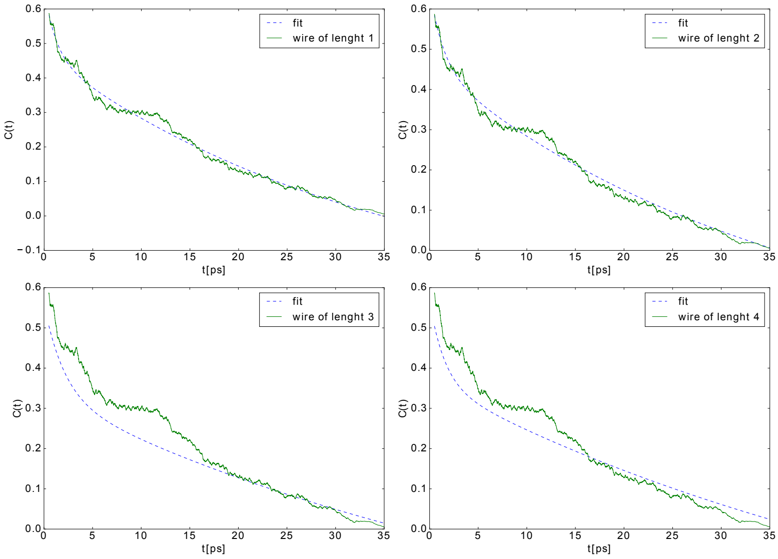


Figure S8: Decorrelation functions for paths of length 1 to 4 (continuous line), as well as the two exponential decay used to fit them (dashed line).

Table S2: Defects along proton wires in simulation A)

| Defect | % path 1 | % path 2 | % path 3 | % path 4 |
|---|---|---|---|---|
| in 1 out 1 | 0.138 | 0.143 | 0.104 | 0.093 |
| in 1 out 2 | 0.388 | 0.151 | 0.116 | 0.135 |
| in 2 out 1 | 0.058 | 0.17 | 0.18 | 0.159 |
| in 2 out 2 | 0.407 | 0.496 | 0.52 | 0.526 |
| in 3 out 2 | 0.002 | 0.021 | 0.046 | 0.053 |

Table S3: Defects along proton wires in simulation D)

| Defect | % path 1 | % path 2 | % path 3 | % path 4 |
|---|---|---|---|---|
| in-1-out-1 | 0.044 | 0.059 | 0.078 | 0.074 |
| in-1-out-2 | 0.152 | 0.22 | 0.215 | 0.172 |
| in-2-out-1 | 0.088 | 0.094 | 0.129 | 0.15 |
| in-2-out-2 | 0.678 | 0.547 | 0.474 | 0.511 |
| in-3-out-2 | 0.031 | 0.058 | 0.078 | 0.065 |
